# Supplementary material for: Extreme field-sensitivity of the magnetic tunneling in Fe-doped Li$_3$N
Source: arXiv:1803.04867 ancillary file (2018-03-13)
Supplement: Supplementary file 1 [file supplement.pdf]

# Supplementary Material: Extreme field-sensitivity of the magnetic tunneling in Fe-doped $Li_3N$

M. Fix,[1] J. H. Atkinson,[2] P. C. Canfield,[3,4] E. del Barco,[2] and A. Jesche[1,*]

[1] *EP VI, Center for Electronic Correlations and Magnetism, Institute of Physics, University of Augsburg, D-86159 Augsburg, Germany*

[2] *Department of Physics, University of Central Florida, Orlando FL 32816, USA*

[3] *The Ames Laboratory, Iowa State University, Ames, Iowa 50011, USA*

[4] *Department of Physics and Astronomy, Iowa State University, Ames, Iowa 50011, USA*

## I ABSENCE OF IN-PLANE MODULATION

Given the sample's SMM-like behavior, attempts were made to find evidence of angular modulation of the QTM splitting at zero-field resonance by measuring the size of the large step at $H_\mathrm{z} = 0$ as a function of the angle of application of a the transverse field within the hard anisotropy plane of the system. This was accomplished by setting a fixed transverse

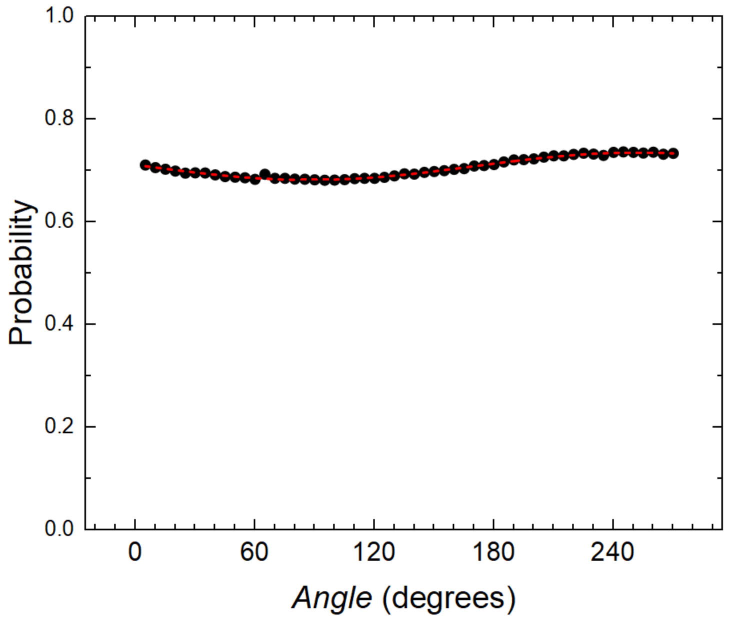


Supplementary Figure 1. Probability of the large step near $H_\mathrm{z} = 0$ as a function of the orientation of a fixed transverse field vector in the xy plane (with 0 degrees $\equiv H_\mathrm{x}$). The red dashed curve is a sine fit, representing the contribution due to a slight misalignment of $H_\mathrm{z}$ with the sample's easy axis. The data was acquired at $T = 230\,\mathrm{mK}$ with a longitudinal field sweep rate of 8.33 mT/s.

.

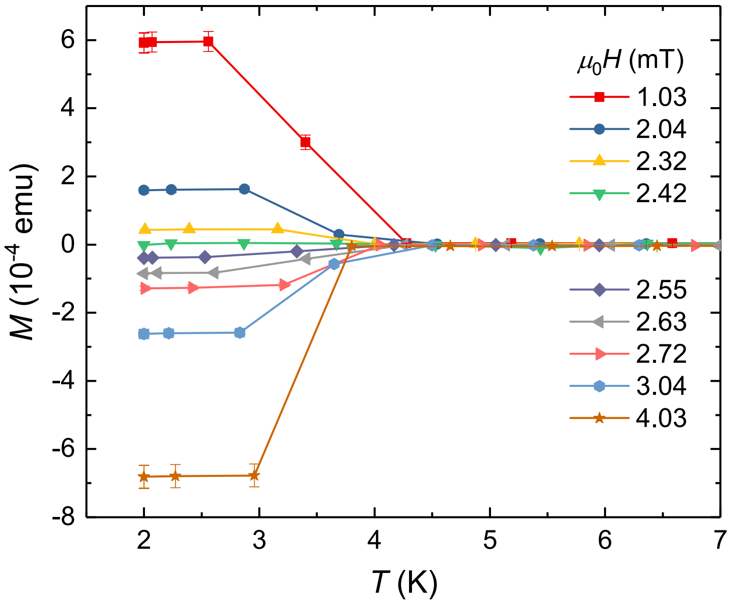


Supplementary Figure 2. Temperature-dependent magnetization of superconducting indium (99.999 %) employed to determine the remnant field of the superconducting magnet of the MPMS3 (lines are guides to the eye). The measurements were performed after ramping the magnet from $\mu_0 H = +7\,\mathrm{T}$ to the nominal values given in the plot. The vanishing magnetization of indium indicates an effective field of $\mu_0 H_{\mathrm{eff}} = (0.0 \pm 0.1)\,\mathrm{mT}$ for a nominal applied field of $\mu_0 H = +2.5\,\mathrm{mT}$.

field vector ($\mu_0|H_{\mathrm{T}}| = 0.02\,\mathrm{T}$ for the data shown in Fig. S1) and sweeping a longitudinal field along $H_{\mathrm{z}}$. The "probability" of the step was then calculated as the fraction of the samples magnetization which relaxed across the feature $(M_{\mathrm{initial}} - M_{\mathrm{final}})/(M_{\mathrm{initial}} - M_{\mathrm{sat}})$. Aside of the one-fold modulation observed in Fig. S1, resulting from a slight misalignment between the field rotation plane and the hard anisotropy plane, the data does not reveal any modulation that could be associated to transverse anisotropy terms in the Hamiltonian governing QTM of the Fe spins. This does not mean that those terms do not exist. It is likely that the zero-field resonance is not sensitive enough to such modulation within the resolution of our technique.

## II REMNANT FIELD OF THE MPMS3 MAGNET

In order to determine the remnant field of the superconducting MPMS3 magnet we measured the temperature dependence of a rod shaped, superconducting indium sample delivered by Quantum Design (99.999 %, The Indium Corporation of America) (see Fig. S2). Prior to the measurement, the magnet was treated identically to the FC measurements of the

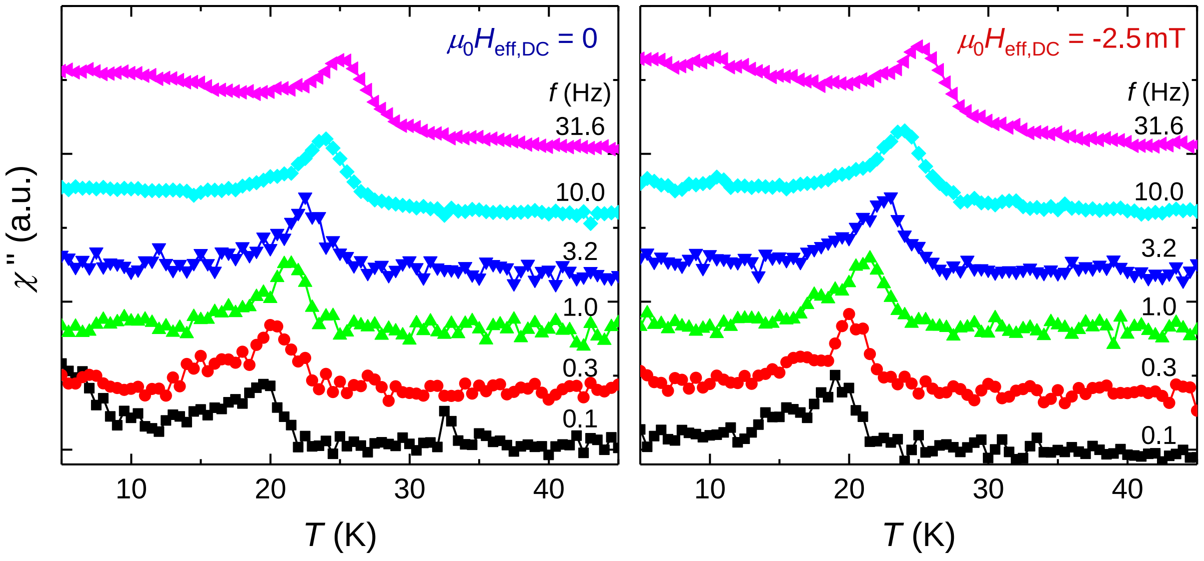


Supplementary Figure 3. Temperature dependence of the out-of-phase magnetic ac susceptibility $\chi''$ of single crystalline $Li_2(Li_{0.999}Fe_{0.001})N$ (curves shifted for clarity, lines are guides to the eye). The ac excitation and an additional static, magnetic field were applied along the crystallographic c-axis. The effective, static magnetic field amounts to $\mu_0 H_{\mathrm{eff,DC}} = 0$ (left panel) and $\mu_0 H_{\mathrm{eff,DC}} = -2.5\,\mathrm{mT}$ (right panel).

$Li_2(Li_{0.999}Fe_{0.001})N$ sample: It was ramped (at $T = 8\,\mathrm{K}$) from $\mu_0 H = +7\,\mathrm{T}$ to the respective fields indicated in Fig. S2 at a rate of 70 mT/s. The magnetization of the In sample was subsequently measured during cooling of the sample to 2 K. The superconducting transition at 3.4 K [1] is apparent and the curves are basically symmetric around the data recorded at the applied fields of $\mu_0 H = 2.42\,\mathrm{mT}$ and 2.55 mT. This measurement was repeated several times with a reproducible outcome. We therefore conclude that ramping the magnet from $\mu_0 H = +7\,\mathrm{T}$ to 2.5(1) mT leads to an effective field of $\mu_0 H_{\mathrm{eff}} = (0.0 \pm 0.1)\,\mathrm{mT}$, compensating for the remnant field of the superconducting magnet.

## III AC SUSCEPTIBILITY

Figure S3 shows the out-of-phase contribution to the alternating current (ac) magnetic susceptibility $\chi''$ versus temperature. The measurement was performed on a single crystal of $Li_2(Li_{0.999}Fe_{0.001})N$. The Fe concentration $x$ was inferred from the known saturation magnetization [2] (crosschecked on other samples by inductively-coupled-plasma optical-emission-spectroscopy measurements). The data were recorded with an ac excitation field of $\mu_0 h_{\mathrm{ac}} = 1.0\,\mathrm{mT}$, applied parallel to the crystallographic c-axis, $h_{\mathrm{ac}} \parallel c$ (curves shifted for

clarity). Owing to the low Fe-concentration, the signal-to-noise ratio becomes too small to allow for an accurate data analysis for frequencies $f > 32\,\mathrm{Hz}$. The relaxation times were determined as $\tau = 1/(2\pi f)$.

## IV ANALYSIS OF THE TIME-DEPENDENCE OF THE MAGNETIZATION

The data obtained from measurements of the relaxation of the magnetization were corrected for the diamagnetic sample holder: The sample was sandwiched between two torlon discs and fixed inside a straw. For the data measured from a saturated state of the magnetization (FC, see main article Fig. 2) the magnetic moment of the sample holder - determined separately in identical configuration - was directly subtracted. For the ZFC measurements in small applied fields starting from $H = 0$ (see main article Fig. 3) the raw data of the DC-measurement of the sample holder was subtracted, followed by fitting the dipole response function of the SQUID-magnetometer to the obtained data.

The diamagnetic contribution of the $Li_3N$ host was subsequently subtracted using $\chi_{\mathrm{M}}(\mathrm{Li}^{1+}) = -8.8 \cdot 10^{-12}\,\mathrm{m^3 mol^{-1}}$ [3] and $\chi_{\mathrm{M}}(\mathrm{N}^{3-}) = -1.63 \cdot 10^{-10}\,\mathrm{m^3 mol^{-1}}$ [4].

Figure S4 shows the resulting time dependent ZFC magnetization in external fields applied parallel and anti-parallel to the c-axis. The symmetry of the curves indicates well defined applied fields close the the nominal values given on the right hand side of the plot. In accordance with the indium measurements (see Sec. 2), the applied field is controlled with an accuracy of $\pm 0.1\,\mathrm{mT}$. The obtained curves were fitted to a stretched exponential function:

$$M = M_{\mathrm{eq}} + (M_0 - M_{\mathrm{eq}}) \exp\left\{ -\left(\frac{t}{\tau}\right)^{\beta} \right\} + M_{\mathrm{off}}, \quad (1)$$

with the equilibrium magnetization $M_{\mathrm{eq}}$, an initial magnetization $M_0$ and $\tau$ is the relaxation time. The exponent $\beta = 0.0 - 1.0$ describes a deviation of the relaxation rate from exponential time-dependence with faster relaxation at early times and the offset $M_{\mathrm{off}}$ accounts for small, time-independent shifts. For the analysis of the FC data, $M_{\mathrm{eq}}$ and $M_{\mathrm{off}}$ were fixed to zero, leaving the 3 free parameters $M_0$, $\tau$ and $\beta$. For the ZFC case, $M_0$ was set to zero. In order to reduce the number of free parameters, $M_{\mathrm{eq}}$ was calculated assuming a two-level system with $\mu_z = \pm 5\,\mu_{\mathrm{B}}$ [2, 5] and $M_{\mathrm{eq}} = 5\mu_{\mathrm{B}} \tanh[(5\mu_{\mathrm{B}} B)/(k_{\mathrm{B}} T)]$. The 3 free parameters in this case are $\tau$, $\beta$ and $M_{\mathrm{off}}$.

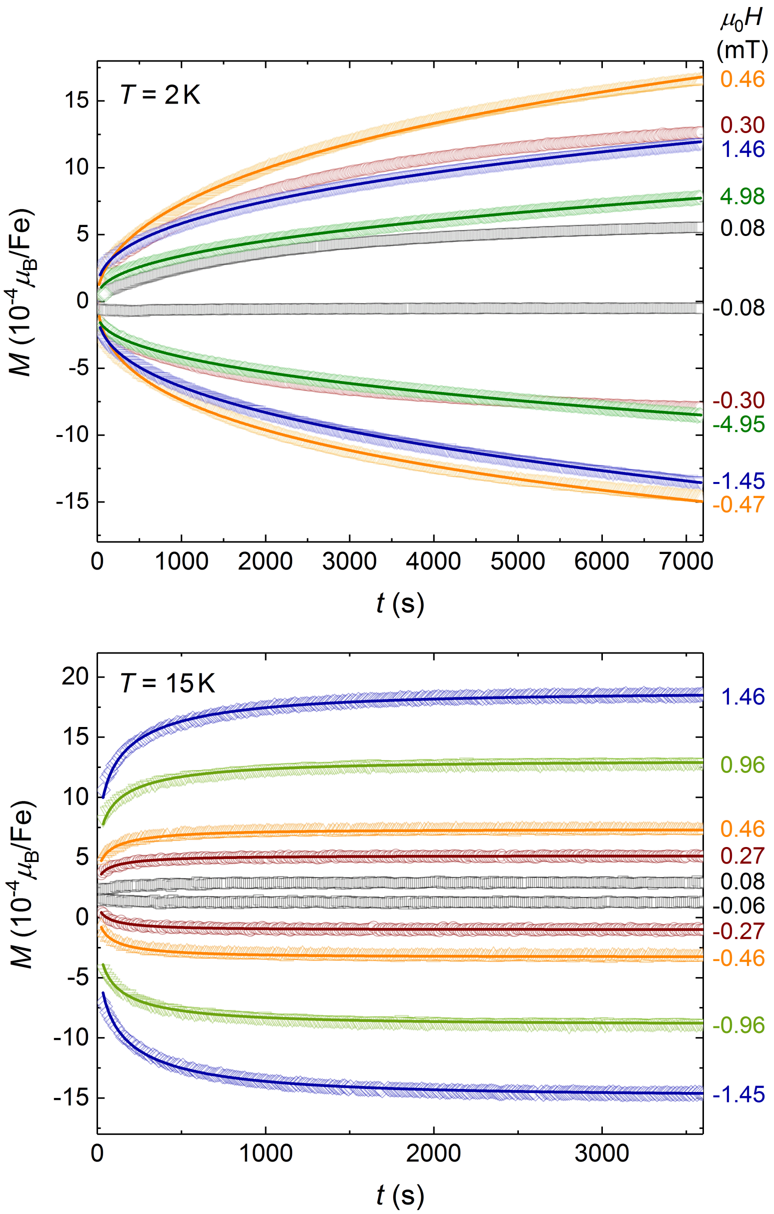


Supplementary Figure 4. Time dependent magnetization as a response to a longitudinal applied field after zero-field-cooling ($H \parallel M \parallel c$) at temperatures of $T = 2\,\mathrm{K}$ (upper panel) and $T = 15\,\mathrm{K}$ (lower panel). The lines are fits to a stretched exponential function (Eq. S1). The curves for parallel and anti-parallel applied fields are basically symmetric, which indicates well defined field values close to the nominal ones (indicated on the right hand side).

## Discussion of the fit parameters

The relaxation times obtained from ZFC measurements at various temperatures are shown in Fig. S5. A continuous development of the peak in $\tau(H)$ can be seen as the sample is cooled from $T = 16\,\mathrm{K}$ to $T = 2\,\mathrm{K}$. Figure S6 shows the field dependence of the other two

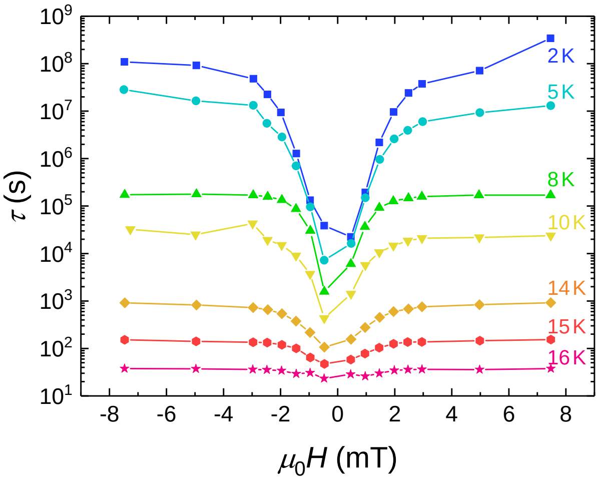


Supplementary Figure 5. Field dependent relaxation times $\tau$ obtained from a fit of Eq. 1 to the ZFC data as described in the text (lines are guides to the eye).

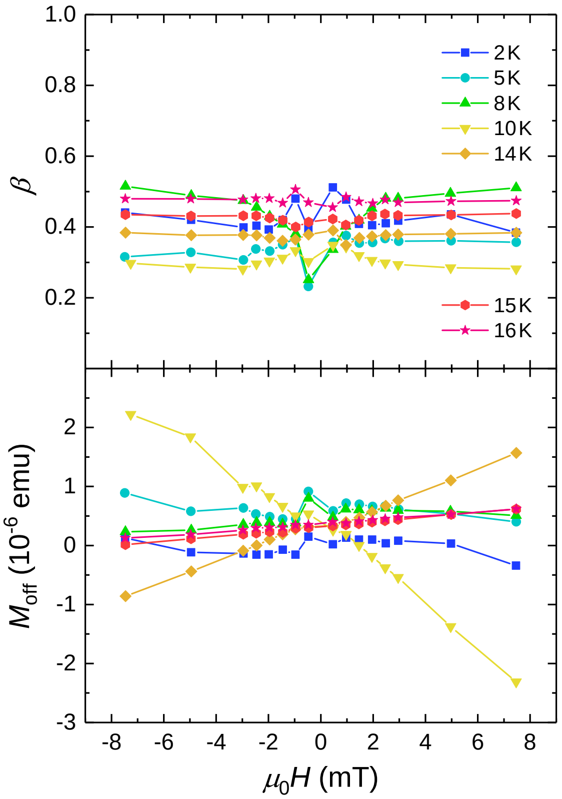


Supplementary Figure 6. Parameters $\beta$ (upper panel) and $M_{\mathrm{off}}$ (lower panel) resulting from a fit of Eq. 1 to the ZFC data (lines are guides to the eye).

fit parameters $\beta$ and $M_{\mathrm{off}}$ for the ZFC measurement. $\beta$ is in the range of $\sim 0.3 - 0.5$ for all temperatures and applied fields and the offset only a small correction ($M_{\mathrm{off}} < 3\,\% M_{\mathrm{eq}}$ for all fits). There is no obvious correlation between the peak found in $\tau(H)$ and the other fit parameters.

Figure S7 shows the temperature dependence of the fit parameter $\beta$ for the FC measurements. The small and essentially temperature independent value of $\beta$ for $T < 10\,\mathrm{K}$ indicates a strong deviation from exponential relaxation of the magnetization in the tunneling regime. $\beta \rightarrow 1$ for higher temperatures in accordance with the transition to the thermally activated relaxation regime where $M \propto \exp(-t/\tau)$.

A comparison of the relaxation times obtained from the two different methods, i.e. from ZFC and FC measurements, respectively is shown in Fig. S8. Since the relaxation in zero applied field is not available from ZFC measurements, we extracted $\tau$ from the smallest applied field that allowed for a reasonable, converging fit, that is for $\mu_0 H = -0.5\,\mathrm{mT}$. The

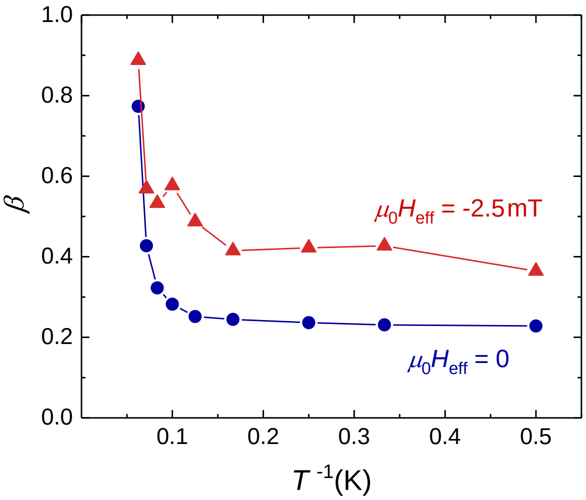


Supplementary Figure 7. Exponent $\beta$ of the stretched exponential function (Eq. 1), determined from a fit to the FC data (lines are guides to the eye).

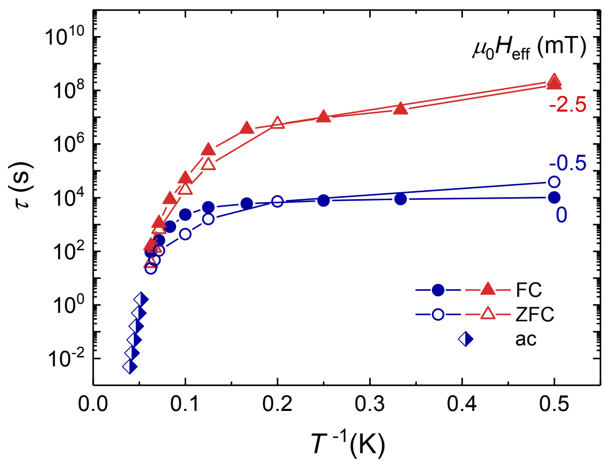


Supplementary Figure 8. Comparison of the relaxation times $\tau$, determined from FC (closed symbols) and ZFC measurements (open symbols) as well as ac susceptibility (diamonds). The lines are guides to the eye.

remarkable agreement of the relaxation times extracted from the two different measurement techniques indicates that fits of $M(T)$ to stretched exponential functions yield a reliable estimate of $\tau$ over 7 orders of magnitude.

* anton.jesche@physik.uni-augsburg.de

[1] L. D. Jennings and C. A. Swenson, Phys. Rev. **112**, 31 (1958).

[2] A. Jesche, R. W. McCallum, S. Thimmaiah, J. L. Jacobs, V. Taufour, A. Kreyssig, R. S. Houk, S. L. Bud'ko, and P. C. Canfield, Nat. Commun. **5:3333** (2014), doi: 10.1038/ncomms4333.

[3] J. Banhart, H. Ebert, J. Voitländer, and H. Winter, J. Magn. Magn. Mater. **61**, 221 (1986).

[4] P. Höhn, S. Hoffmann, J. Hunger, S. Leoni, F. Nitsche, W. Schnelle, and R. Kniep, Chem. Eur. J. **15**, 3419 (2009).

[5] L. Xu, Z. Zangeneh, R. Yadav, S. Avdoshenko, J. van den Brink, A. Jesche, and L. Hozoi, Nanoscale , DOI: 10.1039/c7nr03041j (2017).
